# Supplementary material for: Weyl magnons in noncoplanar stacked kagome antiferromagnets
Source: arXiv:1708.04240 source file (2018-03-01)
Supplement: Supplementary file 1 [file WM_AHE_SM.pdf]

# Supplemental Material for Weyl magnons in noncoplanar stacked kagomé antiferromagnets

S. A. Owerre[1]

[1] *Perimeter Institute for Theoretical Physics, 31 Caroline St. N., Waterloo, Ontario N2L 2Y5, Canada.*

(Dated: October 19, 2017)

The purpose of this Supplemental Material is to show that the in-plane Dzyaloshinskii-Moriya interaction (DMI) provides the same noncoplanar spin canting as the external magnetic field considered in the Main Text. We will also compute the topological (anomalous) thermal Hall effect due to Weyl magnons at the lowest excitation.

## I. INTRODUCTION

In the classical Hall effect [1], a magnetic field is applied perpendicular to the direction of an electric current in metals and causes charge carriers to experience a Lorentz force. The propagation of electric current is deflected in circular orbits by the Lorentz force and charges accumulate on the edge of the material which causes a voltage difference called the Hall voltage. Quantum mechanically, the circular orbits can be quantized as Landau levels and give rise to a quantized Hall conductivity termed the integer quantum Hall effect [2–7]. The anomalous Hall effect arises from the quantum Berry curvature due to nontrivial electronic band topology [8]. It can manifest spontaneously and scales with the magnetization in ferromagnets. Recently, the anomalous Hall effect has been reported in zero magnetic-field antiferromagnets with strong spin-orbit coupling (SOC) and vanishingly small magnetization [9–16]. It can also manifest as a topological Hall effect resulting from nontrivial noncoplanar chiral spin textures [17–21] even in the absence of SOC. Its quantized form is termed the quantum anomalous Hall effect [22–24].

The anomalous thermal Hall effect also requires the presence of a Berry curvature similar to the anomalous Hall effect, but in this case a transverse heat current flows under the influence of a longitudinal thermal gradient. In contrast to electronic charged particles, the carriers of the anomalous thermal Hall effect in magnetic systems are charge-neutral bosonic quasiparticles such as magnons, phonons, triplons, and spinons, and they do not experience a Lorentz force, but the Berry curvature can be regarded as an effective magnetic field in momentum space. In insulating quantum ferromagnets the presence of spontaneous magnetization together with an out-of-plane Dzyaloshinskii-Moriya (DM) interaction [25, 26] (or SOC) in the direction of the magnetization breaks time-reversal symmetry (TRS) and generates a nonzero Berry curvature [27–34], which induces an anomalous thermal Hall effect [27–33, 35–37]. This effect has also been observed in frustrated magnets with spin liquid states [38, 39], and recently in multiferroics [40]. To date, however, the anomalous thermal Hall effect has not been observed experimentally in magnetically ordered insulating antiferromagnets with vanishingly small magnetization. To our knowledge, there is no theoretical or experimental study of the anomalous thermal Hall effect induced by Weyl magnons (WMs).

The insulating quantum antiferromagnets are of great interest and they behave differently from insulating quantum ferromagnets. For example, in frustrated kagomé antiferromagnets with only an out-of-plane DM interaction, a conventional non-collinear 120° magnetic structure with zero scalar spin chirality can be induced. It possesses an effective TRS and leads to vanishing Berry curvature, thus forbids an anomalous thermal Hall effect. This scenario is strikingly different from ferromagnets where the out-of-plane DM interaction inevitably leads to an anomalous thermal Hall effect [27, 28, 30–32, 35–37]. Interestingly, most frustrated kagomé antiferromagnets intrinsically possess both in-plane and out-of-plane DM interactions. While the out-of-plane DM component stabilizes a non-collinear 120° spin structure, the in-plane DM component induces canting out-of-plane and leads to a noncoplanar chiral spin structure with nonzero scalar spin chirality, which breaks TRS macroscopically [41–47]. A non-negligible interlayer coupling establishes a three-dimensional (3D) spin structure. Therefore, we expect that WMs and the associated anomalous thermal Hall effect should exist in 3D stacked frustrated kagomé antiferromagnets even with vanishingly small magnetization.

In this Supplemental Material, we show that the topological (anomalous) thermal Hall effect is indeed present in 3D stacked frustrated kagomé antiferromagnets with WM nodes. The original proposal of WMs in this system is given in the main text, albeit at zero in-plane DM interaction and nonzero magnetic field. In the current study, we consider the effects of both the in-plane and out-of-plane DM interactions at zero magnetic field. The presence of an in-plane DM interaction at zero magnetic field provides an intrinsic property of the WMs in this system, which leads to intrinsic topological (anomalous) thermal Hall effect. Moreover, the WMs in this system are different from those of pyrochlore antiferromagnets [49, 50] by the presence of the scalar spin chirality of noncoplanar chiral spin texture. Therefore, they are provided by explicit macroscopically broken TRS as opposed to implicit broken TRS by the magnetic order in pyrochlore antiferromagnets. Another issue with WMs in pyrochlore antiferromagnets [49, 50] is that they appear in the absence of the DM interaction, however gapped topological magnon bands were recently found in pyrochlore anti-

ferromagnets with DM interaction [51], which suggests that the WMs in pyrochlore antiferromagnets could be gapped out by the DM interaction. In addition, the WMs in pyrochlore (anti)ferromagnets [49, 52, 53] occur above the lowest excitation at high energy. However, in any bosonic system the lowest excitation is thermally populated at low temperatures due to the Bose function, and makes dominant contributions to the thermal Hall conductivity [27–29]. Hence, due to the population effect the WMs in pyrochlore (anti)ferromagnets [49, 52, 53] will not contribute to the anomalous thermal Hall effect at low temperatures. Therefore, previous experimentally reported thermal Hall conductivity in pyrochlore ferromagnets [35, 36] and a subsequent theoretical calculation [29] are definitely not a consequence of recently proposed WMs in this system [52, 53].

The most important property of WMs in the current model is that they come from the lowest magnon excitation, hence they contribute significantly to the thermal Hall conductivity at low temperatures. In this regard, it is valid to say that the most important WM nodes with potential applications are definitely those in the lowest excitation [54]. We show that the topological (anomalous) thermal Hall effect of WMs in this system depends on the distribution and distance between the WM nodes in momentum space. In general, the thermal Hall conductivity is a 3-pseudo-vector $\left(\kappa_{yz}^x, \kappa_{zx}^y, \kappa_{xy}^z\right)$, however the first two components vanish because the distribution of the WM nodes in momentum space comes in pairs of opposite chiralities and leads to zero net Berry curvature in the plane perpendicular to the $k_x$ or $k_y$ momentum direction. But the plane perpendicular to the out-of-plane $k_z$ momentum direction contains WMs with nonzero net Berry curvature across the planes, which yields a finite $\kappa_{xy}^z$. The 3D thermal Hall conductivity can be separated as

$$\kappa_{xy}^z = \int_{-\pi}^{\pi} \frac{dk_z}{2\pi} \kappa_{xy}^{\text{2D}}(k_z), \tag{1}$$

where $\kappa_{xy}^{\text{2D}}(k_z)$ is a set of 2D thermal Hall conductivity in the $k_x$-$k_y$ plane [30] parameterized by $k_z$. It is given by

$$\kappa_{xy}^{\text{2D}}(k_z) = -T \int \frac{d\mathbf{k}_\parallel}{(2\pi)^2} \sum_{n=1}^{N} c_2\left(f^B[E_n(\mathbf{k}_\parallel, k_z)]\right) \Omega_{n\mathbf{k}_\parallel}^z(k_z), \tag{2}$$

where $\mathbf{k}_\parallel = (k_x, k_y)$, $T$ is the temperature, $c_2$ is a function of the Bose function and $\Omega_{n\mathbf{k}_\parallel}^z(k_z)$ is the Berry curvature. Since the Berry curvature is dominant near the WM nodes, the major contribution to the thermal Hall conductivity comes from these nodes at the lowest magnon band due to the Bose function. Hence, at $T \neq 0$ the empirical expression for the topological (anomalous) thermal Hall conductivity can be written as

$$\kappa_{xy}^z \propto \sum \Delta k_0^i, \tag{3}$$

where $\Delta k_0^i$ is the separation of the WM nodes along the $k_z$ momentum direction, which depends on the scalar spin chirality of noncoplanar chiral spin texture induced by the in-plane DM interaction. This relation is akin to the anomalous Hall conductivity in electronic Weyl semimetal [55, 56]. Indeed, when the WM nodes annihilate at the Brillouin zone (BZ) boundary, the system becomes a fully gapped 3D topological magnon insulator with similar features to 2D counterparts [57–60].

## II. SPIN MODEL

At zero magnetic field, 3D stacked kagomé-lattice antiferromagnets are governed by the Hamiltonian

$$\mathcal{H} = J \sum_{\langle ij\rangle,\ell} \mathbf{S}_{i,\ell} \cdot \mathbf{S}_{j,\ell} + \sum_{\langle ij\rangle,\ell} \mathbf{D}_{ij} \cdot \mathbf{S}_{i,\ell} \times \mathbf{S}_{j,\ell} + J_c \sum_{i,\langle \ell\ell'\rangle} \mathbf{S}_{i,\ell} \cdot \mathbf{S}_{i,\ell'}, \tag{4}$$

where $i$ and $j$ denote nearest neighbour sites on the kagomé layers, $\ell$ and $\ell'$ label the layers. The first term is the intralayer antiferromagnetic Heisenberg exchange interaction. The second term is the DM interaction [25, 26] due to lack of inversion symmetry between two sites on each layer. Using the convention in ref. 41 we take $\mathbf{D}_{ij} = (D_p \cos\varphi, D_p \sin\varphi, D_z)$, where $\varphi$ is the angle between the projection of the spin and the kagomé plane. The orientations of the in-plane and out-of-plane DM vectors $D_p$ and $D_z$ respectively are depicted in Fig. 1. The out-of-plane DM component $D_z > 0$ stabilizes a $120^\circ$ non-collinear spin configuration with positive vector chirality and retain U(1) rotational invariance about the out-of-plane $z$ direction, whereas the in-plane DM component $D_p$ induces canting out-of-plane and leads to a noncoplanar chiral spin structure with broken time-reversal and rotational symmetries [41–47]. The last term is an unshifted interlayer antiferromagnetic interaction that establishes a 3D spin structure. The most important physical consequence of this model is that all the interactions are allowed in real kagomé antiferromagnetic materials. For $\varphi = 0$ the classical ground state energy is given by

$$E_{\text{cl}} = -3NS^2\Big[J\left(1 - 3\sin^2\eta\right) + \sqrt{3}D_z\cos^2\eta + \sqrt{3}D_p\sin 2\eta + J_c\cos 2\eta\Big], \tag{5}$$

where $N$ is the number of sites per unit cell, $S$ is the spin value, and $\eta$ is the canting angle induced by $D_p$. The classical energy is minimized by

$$\tan 2\eta = \frac{2\sqrt{3}D_p}{3J + \sqrt{3}D_z + 2J_c}. \tag{6}$$

Evidently, the in-plane DM interaction provide similar spin canting as an external magnetic field [48], and leads

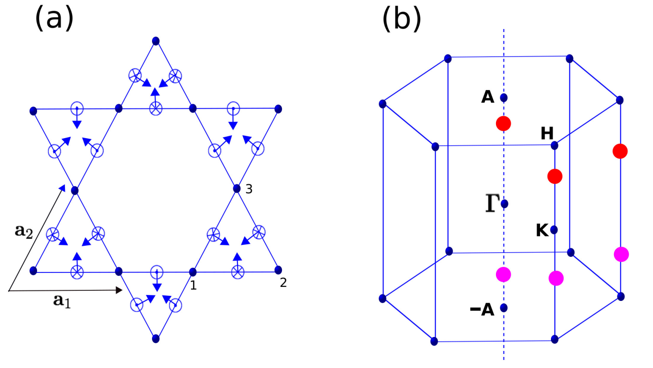


FIG. 1: Color online. (a). Top view of kagomé layers stacked perfectly along the (001) direction. It contains in-plane (arrows) and out-of-plane (dotted and crossed circles) DM interactions. The numbers $(1, 2, 3)$ label the sublattices. The in-plane unit vectors are $\mathbf{a}_1 = (1, 0, 0)$ and $\mathbf{a}_2 = (1/2, \sqrt{3}/2, 0)$. The unit vector along the stacking direction $\mathbf{a}_3 = (0, 0, 1)$ is not depicted. (b). The 3D Brillouin zone. Red and pink dots denote the locations of the lowest excitation WM nodes with opposite chiralities along the $k_z$ momentum direction.

to noncoplanar chiral spin structure with nonzero scalar spin chirality (see Appendix). For decoupled kagomé planes i.e. $J_c = 0$, we recover the canting angle of single layer kagomé lattice in ref. 41.

## III. MAGNON BAND FEATURES

### A. Weyl magnons

We now study the WM bands in the current model. As we pointed out above, at zero magnetic field the in-plane DM interaction induces similar spin canting (scalar spin chirality) a nonzero magnetic field induces at zero in-plane DM interaction [48]. The major difference here is that the in-plane DM interaction is intrinsic to kagomé materials and breaks rotational symmetry. Hence, the current model have gapped modes at $\mathbf{k} = (k_x, k_y, k_z) = 0$. In order to study the magnon bands in this model, we generalize linear spin wave theory of 2D kagomé-lattice antiferromagnets with in-plane and out-of-plane DM interaction [61, 62] to 3D unshifted stacked kagomé-lattice antiferromagnets. The basic procedures are outlined in the Appendix. At $D_p = 0$ and $D_z \neq 0$ the ground state of the Hamiltonian (4) is a 3D conventional non-collinear $120°$ magnetic structure with zero scalar spin chirality. Hence, TRS is broken only by the magnetic order but not macroscopically. In this limit degenerate magnon bands form nodal-line magnons (NLMs) as previously shown [48]. A nonzero $D_p \neq 0$ induces 3D noncoplanar chiral spin texture with non-zero scalar spin chirality which breaks TRS macroscopically. Similar to the magnetic field model [48], the degeneracy of the magnon bands are lifted and the NLMs are gapped everywhere except at the WM nodes located at $(\pm 2\pi/3, 0, \pm k_0^1)$ and $(0, 0, \pm k_0^2)$. At $(k_x, k_y) = (\pm 2\pi/3, 0)$ and $(k_x, k_y) = (0, 0)$ the eigenvalues of the Bogoliubov spin wave Hamiltonian can be found exactly as a function of $k_z$, hence the locations of the WM nodes $k_0^{1(2)}$ (see Appendix). We have shown the WM bands along the $k_z$ directions in Fig. 2 in the weakly coupled regime $J_c < J$ and strongly coupled regime $J_c \geq J$. A distinguishing feature of this model is that without the lowest magnon band the middle and topmost magnon band never cross each other. Therefore the WM nodes comes from the lowest excitations. In the weakly coupled regime $J_c < J$ the WM nodes at $(\pm 2\pi/3, 0, \pm k_0^1)$ are more dominant than those at $(0, 0, \pm k_0^2)$, whereas in the strongly coupled regime $J_c \geq J$ those at $(0, 0, \pm k_0^2)$ are more dominant than those at $(\pm 2\pi/3, 0, \pm k_0^1)$ (see the chiral magnon surface states below). Also note that WM nodes exist for any nonzero $D_z$ and $D_p$, with a non-negligible interlayer antiferromagnetic interaction $J_c$. Due to broken rotational invariance induced by $D_p \neq 0$ the lowest mode is gapped at $\mathbf{k} = 0$.

### B. Berry curvature

The interesting properties of WMs and the anomalous thermal Hall effect are manifested in the Berry curvature. As shown in the Appendix, once we diagonalize the spin wave Bogoliubov Hamiltonian $\mathcal{H}_B(\mathbf{k})$, the Berry curvature of a given magnon band $n$ can be defined as

$$\Omega^{\gamma}_{n,\alpha\beta}(\mathbf{k}) = -\sum_{m\neq n} \frac{2\text{Im}[\langle \mathcal{P}_{\mathbf{k}n}|\hat{v}_\alpha|\mathcal{P}_{\mathbf{k}m}\rangle \langle \mathcal{P}_{\mathbf{k}m}|\hat{v}_\beta|\mathcal{P}_{\mathbf{k}n}\rangle]}{\left(E_n(\mathbf{k}) - E_m(\mathbf{k})\right)^2}, \tag{7}$$

where $\hat{v}_\alpha = \partial \mathcal{H}_B(\mathbf{k})/\partial k_\alpha$ defines the velocity operators and $\alpha, \beta, \gamma = x, y, z$. $\mathcal{P}_{\mathbf{k}n}$ are the paraunitary operators (eigenvectors) that diagonalize $\mathcal{H}_B(\mathbf{k})$ and $E_n(\mathbf{k})$ are the eigenvalues. Note that the Berry curvature is a 3-pseudo-vector pointing along the $\gamma$ directions perpendicular to both the $\alpha$ and $\beta$ directions. The WM nodes come in pairs of opposite chiralities, and act as source (monopole) and sink (antimonopole) of the Berry curvature. We have confirmed this in Fig. 3 (Top panel), where the red and pink circles denote $\pm 1$ chirality respectively.

### C. Magnon arc surface states

One of the hallmarks of WMs is the chiral magnon arc surface states (SS), which connect projected WM nodes with opposite chiralities on any surface in momentum space not perpendicular to the $k_z$ direction. To show this, we consider a slab on the $k_y = 0$ plane with open boundary conditions along $x$ direction and infinite along $z$ direction. Indeed, as shown in Fig. 3 (Bottom panel) two projected WM nodes on the $k_y = 0$ plane along the $k_z$ direction with opposite chiralities $\pm 1$ are connected by a chiral magnon arc SS. This is consistent with the

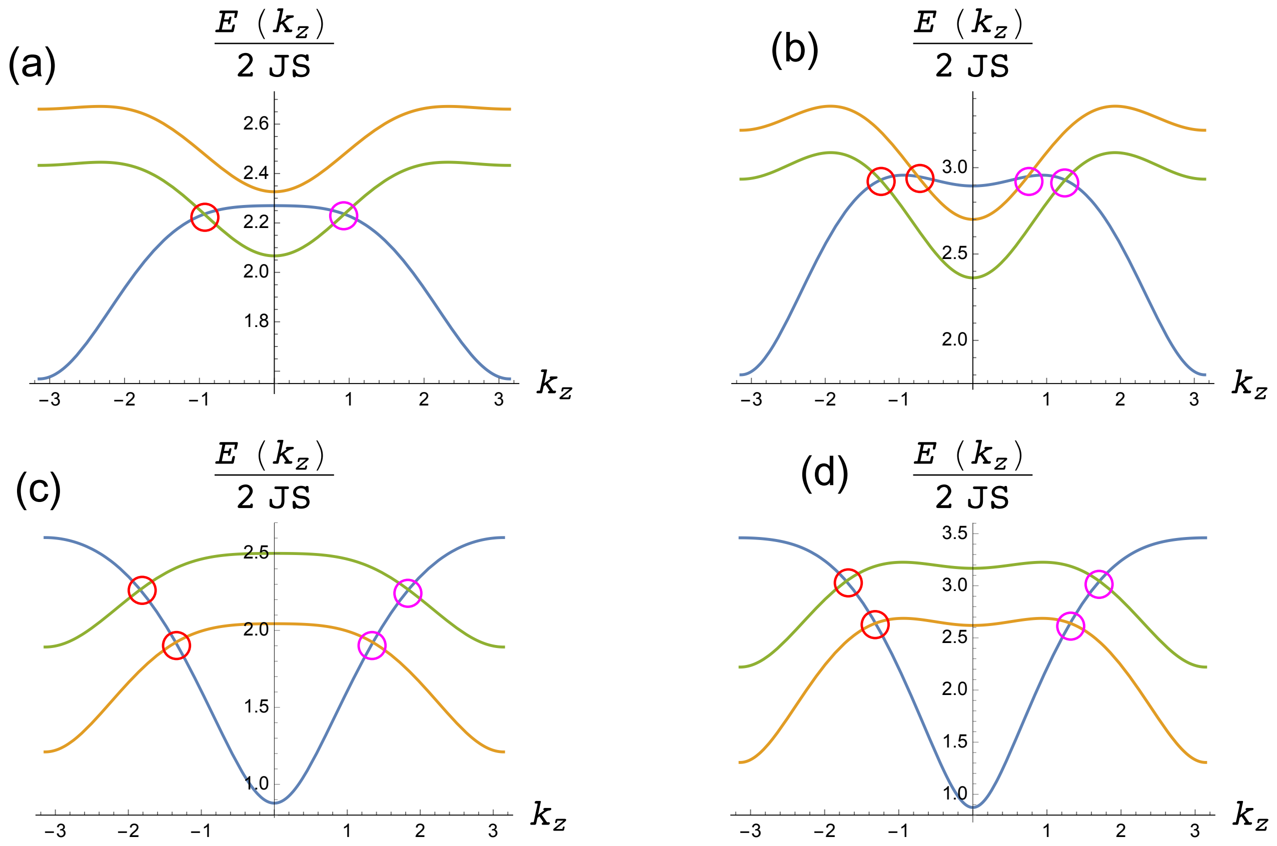


FIG. 2: Color online. Weyl magnon bands along the $k_z$ direction for $D_z/J = 0.3$, $D_p/J = 0.5$. Top panel $(k_x, k_y) = (2\pi/3, 0)$. (a). $J_c/J = 0.8$ (b). $J_c/J = 1.5$. Bottom panel $(k_x, k_y) = (0, 0)$. (c). $J_c/J = 0.8$ (d). $J_c/J = 1.5$. The WM nodes are highlighted with red and pink circles.

monopole – antimonopole distribution of the WMs in Fig. 3 (Top panel).

## IV. TOPOLOGICAL THERMAL HALL EFFECT

Now, we turn to the main purpose of this report — the topological (anomalous) thermal Hall effect due to WMs. As we mentioned above, the topological or anomalous thermal Hall effect induced by WMs has not been studied both theoretically and experimentally. We will provide a theoretical description in this section. The thermal Hall effect is due to flow of heat current $J_\alpha^\gamma$ under the influence of a thermal gradient $\nabla_\beta T$. It can be derived from linear response theory [28, 30]. The total intrinsic anomalous thermal Hall conductivity can be written as $\kappa_H = \left(\kappa_{yz}^x + \kappa_{zx}^y + \kappa_{xy}^z\right)/3$, where the components $\kappa_{\alpha\beta}^\gamma = -J_\alpha^\gamma/\nabla_\beta T$ are given explicitly by

$$\kappa_{\alpha\beta}^\gamma = -T\int_{BZ}\frac{d\mathbf{k}}{(2\pi)^3}\sum_{n=1}^{N} c_2\left(f_n^B\right)\Omega_{n,\alpha\beta}^\gamma(\mathbf{k}), \tag{8}$$

where $f_n^B = \left(e^{E_n(\mathbf{k})/T} - 1\right)^{-1}$ is the Bose function with the Boltzmann constant set to unity, and $c_2(x) = (1 + x)\left(\ln\frac{1+x}{x}\right)^2 - (\ln x)^2 - 2\text{Li}_2(-x)$, with $\text{Li}_2(x)$ being the dilogarithm. Evidently, the anomalous thermal Hall conductivity is the integration of the Berry curvature over the BZ, weighed by the $c_2$ function. Due to the Berry curvature, $\kappa_{\alpha\beta}^\gamma$ is also a 3-pseudo-vector pointing along the $\gamma$ directions perpendicular to both the $\alpha$ and $\beta$ directions. For $D_p = 0$ and $D_z \neq 0$ the 3D conventional non-collinear 120° magnetic structure has an effective TRS defined as the combination of TRS ($\mathcal{T}$) and 180° spin rotation of the in-plane spin order about the $z$ direction ($\mathcal{R}_z$), or mirror reflection symmetry of the kagomé plane about the $y$ direction ($\mathcal{M}_y$). Thus, $\Omega_{n,\alpha\beta}^\gamma(\mathbf{k}) = -\Omega_{n,\alpha\beta}^\gamma(-\mathbf{k})$ and $\kappa_{\alpha\beta}^\gamma = 0$. For $D_p \neq 0$ these symmetries are broken leading to noncoplanar chiral spin texture. Therefore $\kappa_{\alpha\beta}^\gamma$ is expected to be nonzero. As the Berry curvature is maximum near the WM nodes, evidently the major contribution to $\kappa_{\alpha\beta}^\gamma$ comes from these nodes. In addition, the presence of Bose function suggests that the lowest magnon band and associated Berry curvature have the dominant contribution to $\kappa_{\alpha\beta}^\gamma$ at low temperature when few magnons are thermally excited. This implies that the most important WM nodes contributing to $\kappa_{\alpha\beta}^\gamma$ must come from the lowest excitation [54].

For any surface not perpendicular to the $k_z$ direction

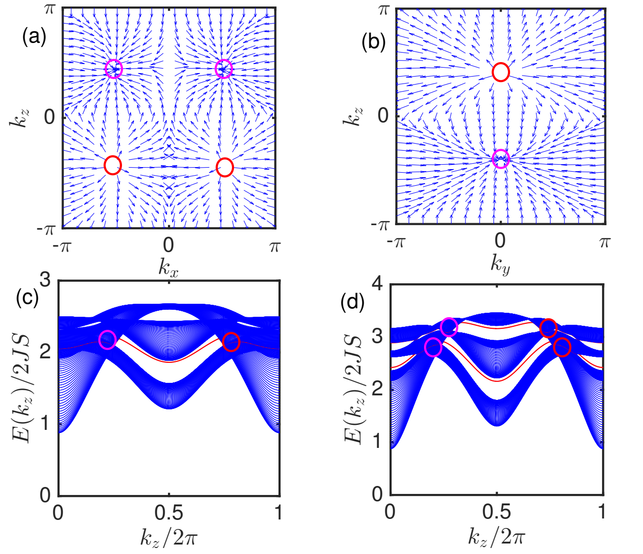


FIG. 3: Color online. Top panel: Monopole and anti-monopole distribution of the lowest magnon band Berry curvature $\Omega^y_{1,xz}(\mathbf{k})$ on the $k_y = 0$ plane (a), and $\Omega^x_{1,yz}(\mathbf{k})$ on the $k_x = 2\pi/3$ plane (b). Here $D_z/J = 0.3$, $D_p/J = 0.5$, $J_c/J = 0.8$. Bottom panel: Two projected WM nodes (red and pink circles) along the $k_z$-axis are connected by a chiral magnon arc SS (red lines) as they have opposite chirality. Here $D_z/J = 0.3$, $D_z/J = 0.5$. (c) $J_c/J = 0.8$ (weakly coupled regime). In this regime the chiral magnon arc SS comes from the WM nodes in Fig. 2(a). (d) $J_c/J = 1.5$ (strongly coupled regime). In this regime the chiral magnon arc SS comes from the WM nodes in Fig. 2(d).

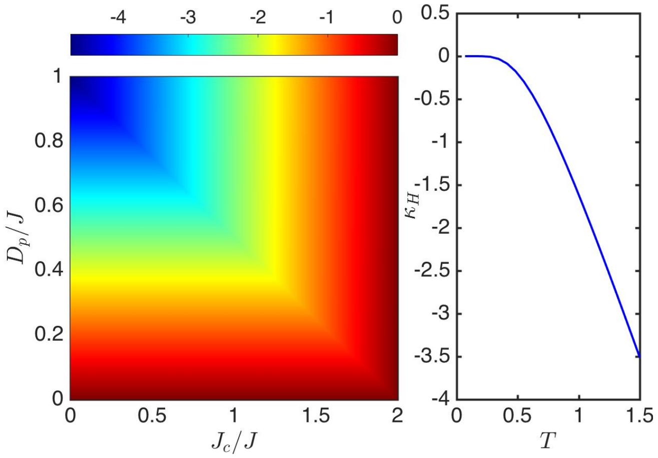


FIG. 4: Color online. Topological (anomalous) thermal Hall conductivity. (Left) Heat map of $\kappa_H \approx \kappa^z_{xy}$ in the $J_c/J$–$D_p/J$ plane at $D_z/J = 0.3$, $T = 0.75$. (Right) $\kappa_H \approx \kappa^z_{xy}$ plotted against $T$ for $D_z/J = 0.3$, $D_p/J = 0.5$, $J_c/J = 0.8$.

the WM nodes come in pairs of opposite chiralities as Fig. 3 shows. Therefore the net Berry curvature vanishes identically. In fact, a direct numerical integration of Eq. 8 shows that $\kappa^x_{yz} = \kappa^y_{zx} \approx 0$. However, for the surface perpendicular to the $k_z$ direction the distributions of WM nodes are different. From the Berry curvature fields in Fig. 3 (Top panel), we see that for fixed $k_z$ in the vicinity of the WM nodes the net Berry curvature in the $k_x$-$k_y$ plane is nonzero. Therefore, integrating over $k_z$ results in nonzero $\kappa^z_{xy}$ as shown in Fig. 4. The anomalous thermal Hall conductivity vanishes at zero temperature as no magnon is thermal excited. It also vanishes at $D_p = 0$ as the scalar spin chirality vanishes, hence TRS is not broken macroscopically. The sign of the anomalous thermal Hall conductivity can be easily switched by a small magnetic field. The anomalous thermal Hall conductivity $\kappa^z_{xy}$ can be separated in two forms as given by Eqs. 1 and 2, from which we infer that empirical formula is given by Eq. 3 at $T \neq 0$, similar to anomalous Hall conductivity in the Weyl semimetal [55, 56]. As the WM nodes annihilate at the BZ boundary, the system becomes a fully gapped 3D topological magnon insulator with also nonzero $\kappa^z_{xy}$, similar to 2D system [57].

## V. CONCLUSION

We have shown that Weyl magnons in three-dimensional noncoplanar stacked frustrated kagomé antiferromagnets possessed a nonzero intrinsic topological (anomalous) thermal Hall effect at zero magnetic field. It is shown that the topological (anomalous) thermal Hall effect depends on the distributions of the Weyl magnon nodes and it is proportional to their distance in momentum space at nonzero temperature. We also showed that the Weyl magnon nodes at the lowest excitation carry the dominant contribution to the topological (anomalous) thermal Hall conductivity at low temperature. Therefore, we have concluded that the most important Weyl magnons in three-dimensional magnetic systems are those at the lowest excitation [54], and they can be easily probed by neutron scattering experiments. The sign of the topological (anomalous) thermal Hall conductivity can be switched by a small external magnetic field, paving the way toward possible applications in magnon spintronics and magnetic data storage devices. Moreover, a nonzero topological (anomalous) thermal Hall conductivity in three-dimensional frustrated kagomé antiferromagnets could also serve as an avenue to probe macroscopically broken time-reversal symmetry or scalar spin chirality. The predicted results can be investigated experimentally by thermal transport measurements.

### Appendix A: Spin transformation

To facilitate spin wave theory we express the spins in terms of local axes, such that the $z$-axis coincides with the spin direction [61, 62]. The transformation matrix is given by

$$\mathcal{R}_t(\theta_{i,\ell}) = \begin{pmatrix} 0 & \sin\theta_{i,\ell} & -\cos\theta_{i,\ell} \\ 0 & \cos\theta_{i,\ell} & \sin\theta_{i,\ell} \\ 1 & 0 & 0 \end{pmatrix}, \tag{A1}$$

where $\theta_{i,\ell}$ are the angles that form 120° non-collinear spin configuration on sublattice $(1,2,3)$ depicted in Fig. 1. Due to spin canting induced by $D_p$ we have to transform the spin from local axes to canting frame using the rotation matrix

$$\mathcal{R}_c(\eta) = \begin{pmatrix} \cos\eta & 0 & -\sin\eta \\ 0 & 1 & 0 \\ \sin\eta & 0 & \cos\eta \end{pmatrix}. \tag{A2}$$

Now, the spins transform as $\mathbf{S}_i = \mathcal{R}_z(\theta_{i,\ell}) \cdot \mathcal{R}_y(\eta) \cdot \mathbf{S}'_i$, where prime denotes the rotated frame.

Note that the triangular plaquettes on the kagomé lattice have $\mathcal{C}_3$ rotational symmetry, hence the bonds $1 \to 2$, $2 \to 3$, and $3 \to 1$ in Fig. 1 have the same coefficients. For instance, for bond $1 \to 2$ the terms that contribute to noninteracting magnon are given by

$$\mathcal{H}_J^{1\to 2} = J\sum_\ell \Big[ -\frac{1}{2}\mathbf{S}'_{1,\ell}\cdot\mathbf{S}'_{2,\ell} - \frac{\sqrt{3}}{2}\sin\eta\hat{\mathbf{z}}\cdot\big(\mathbf{S}'_{1,\ell}\times\mathbf{S}'_{2,\ell}\big) + \frac{3}{2}\big(\cos^2\eta S'^x_{1,\ell}S'^x_{2,\ell} + \sin^2\eta S'^z_{1,\ell}S'^z_{2,\ell}\big)\Big], \tag{A3}$$

$$\mathcal{H}_{D_z}^{1\to 2} = D_z\sum_\ell \Big[\frac{1}{2}\sin\eta\;\hat{\mathbf{z}}\cdot\big(\mathbf{S}'_{1,\ell}\times\mathbf{S}'_{2,\ell}\big) - \frac{\sqrt{3}}{2}\Big(\sin^2\eta S'^x_{1,\ell}S'^x_{2,\ell} + S'^y_{1,\ell}S'^y_{2,\ell} + \cos^2\eta S'^z_{1,\ell}S'^z_{2,\ell}\Big)\Big], \tag{A4}$$

$$\mathcal{H}_{D_p}^{1\to 2} = D_p\sum_\ell \Big[\frac{\sqrt{3}\sin 2\eta}{2}\big(S'^x_{1,\ell}S'^x_{2,\ell} - S'^z_{1,\ell}S'^z_{2,\ell}\big) + \frac{\cos\eta}{2}\hat{\mathbf{z}}\cdot\big(\mathbf{S}'_{1,\ell}\times\mathbf{S}'_{2,\ell}\big)\Big]. \tag{A5}$$

The $\mathcal{C}_3$ rotational symmetry guarantees that bonds $2 \to 3$ and $3 \to 1$ have the same form of Hamiltonians. The interlayer coupling transforms as

$$\mathcal{H}_{J_c} = J_c\sum_{i,\langle\ell\ell'\rangle}\Big[\cos\theta_{\ell\ell'}\mathbf{S}'_{i,\ell}\cdot\mathbf{S}'_{i,\ell'} + 2\sin^2\Big(\frac{\theta_{\ell\ell'}}{2}\Big)\big(\cos^2\eta S'^x_{i,\ell}S'^x_{i,\ell'} + \sin^2\eta S'^z_{i,\ell}S'^z_{i,\ell'}\big)\Big], \tag{A6}$$

where $\theta_{\ell\ell'} = \theta_\ell - \theta_{\ell'}$. Here $\theta_{\ell\ell'} = \pi$ for antiferromagnetic interlayer coupling $J_c > 0$, and $\theta_{\ell\ell'} = 0$ for ferromagnetic interlayer $J_c < 0$. Note that the scalar spin chirality of the noncoplanar (umbrella) spin configurations defined as

$$\chi = \sum_{ijk,l}\mathbf{S}'_{i,\ell}\cdot\big(\mathbf{S}'_{j,\ell}\times\mathbf{S}'_{k,\ell}\big), \tag{A7}$$

is induced only within the kagomé planes. It vanishes at $D_p = 0$ by virtue of the classical ground state energy and the canting angle given by Eqs. 5 and 6 in the main text.

## Appendix B: Holstein-Primakoff transformation

Next, we introduce the Holstein-Primakoff bosons:

$$S^z_{i,\ell} = S - a^\dagger_{i,\ell}a_{i,\ell},\; S^+_{i,\ell} \approx \sqrt{2S}a_{i,\ell} = (S^-_{i,\ell})^\dagger, \tag{B1}$$

where $S^\pm_{i,\ell} = S^x_{i,\ell} \pm iS^y_{i,\ell}$ and $a^\dagger_{i,\ell}(a_{i,\ell})$ are the bosonic creation (annihilation) operators. The resulting magnon tight-binding model is given by

$$\mathcal{H}_{J-D_{z(p)}} = S\sum_{\langle ij\rangle,\ell}\big[t^z(a^\dagger_{i,\ell}a_{i,\ell} + a^\dagger_{j,\ell}a_{j,\ell}) + t^r(e^{-i\phi_{ij,\ell}}a^\dagger_{i,\ell}a_{j,\ell} + h.c.) + t^o(a^\dagger_{i,\ell}a^\dagger_{j,\ell} + h.c.)\big], \tag{B2}$$

$$\mathcal{H}_{J_c} = S\sum_{i,\ell}t^z_c a^\dagger_{i,\ell}a_{i,\ell} + S\sum_{i,\langle\ell\ell'\rangle}\big[t^r_c(a^\dagger_{i,\ell}a_{i,\ell'} + h.c.) + t^o_c(a^\dagger_{i,\ell}a^\dagger_{i,\ell'} + h.c.)\big]. \tag{B3}$$

The parameters of the tight binding model are given by

$$t^z = \frac{J}{2}\big(1 - 3\sin^2\eta\big) + \frac{\sqrt{3}}{2}D_z\cos^2\eta + \frac{\sqrt{3}D_p}{2}\sin 2\eta, \tag{B4}$$

$$t^r = \sqrt{(t^r_1)^2 + (t^r_2)^2}, \tag{B5}$$

$$t^r_1 = \frac{J}{2}\Big[-1 + \frac{3}{2}\cos^2\eta\Big] - \frac{\sqrt{3}D_z}{2}\Big(1 - \frac{\cos^2\eta}{2}\Big) + \frac{\sqrt{3}D_p}{4}\sin 2\eta, \tag{B6}$$

$$t^r_2 = -\frac{1}{2}\big[(\sqrt{3}J - D_z)\sin\eta - D_p\cos\eta\big], \tag{B7}$$

$$t^o = \frac{1}{4}(3J + \sqrt{3}D_z)\cos^2\eta + \frac{\sqrt{3}D_p}{4}\sin 2\eta, \tag{B8}$$

$$t^z_c = 2J_c\cos 2\eta,\; t^r_c = -J_c\sin^2\eta,\; t^o_c = J_c\cos^2\eta. \tag{B9}$$

The solid angle subtended by three noncoplanar spins is given by $\phi_{ij} = \pm\phi$, where $\phi = \tan^{-1}[t^r_2/t^r_1]$. Next, we Fourier transform into momentum space with basis vector $\psi^\dagger_{\mathbf{k}} = (a^\dagger_{\mathbf{k}1}, a^\dagger_{\mathbf{k}2}, a^\dagger_{\mathbf{k}3}, a_{-\mathbf{k}1}, a_{-\mathbf{k}2}, a_{-\mathbf{k}3})$. The resulting Hamiltonian is given by

$$\mathcal{H}(\mathbf{k}) = 2S\begin{pmatrix} \boldsymbol{\mathcal{G}}^0(k_z) + \boldsymbol{\mathcal{G}}^r(k_\parallel) & \boldsymbol{\mathcal{G}}^o(k_\parallel, k_z) \\ \boldsymbol{\mathcal{G}}^o(k_\parallel, k_z) & \boldsymbol{\mathcal{G}}^0(k_z) + \boldsymbol{\mathcal{G}}^r(k_\parallel)\end{pmatrix}, \tag{B10}$$

where $\mathbf{k} = (k_\parallel, k_z)$ and $k_\parallel = (k_x, k_y)$. The $\boldsymbol{\mathcal{G}}$ matrices are given by $\boldsymbol{\mathcal{G}}^0(k_z) = [(t^z_c + 4t^z)/2 + t^r_c\cos k_z]\mathbf{I}_{3\times 3}$

$$\boldsymbol{\mathcal{G}}^r(k_\parallel) = t^r\begin{pmatrix} 0 & \cos k^1_\parallel e^{-i\phi} & \cos k^3_\parallel e^{i\phi} \\ \cos k^1_\parallel e^{i\phi} & 0 & \cos k^2_\parallel e^{-i\phi} \\ \cos k^3_\parallel e^{-i\phi} & \cos k^2_\parallel e^{i\phi} & 0 \end{pmatrix}, \tag{B11}$$

$$\boldsymbol{\mathcal{G}}^o(k_\parallel,k_z)=\begin{pmatrix}t_c^o\cos k_z & t^o\cos k_\parallel^1 & t^o\cos k_\parallel^3\\ t^o\cos k_\parallel^1 & t_c^o\cos k_z & t^o\cos k_\parallel^2\\ t^o\cos k_\parallel^3 & t^o\cos k_\parallel^2 & t_c^o\cos k_z\end{pmatrix}, \quad \text{(B12)}$$

where $k_\parallel^i = k_\parallel\cdot\mathbf{a}_i$, with $\mathbf{a}_1=\hat{x}$, $\hat{\mathbf{a}}_2=\hat{x}/2+\sqrt{3}\hat{y}/2$, and $\hat{\mathbf{a}}_3=-\hat{x}/2+\sqrt{3}\hat{y}/2$. The momentum space Hamiltonian for $J_c<0$ can be derived in a similar way. However, we will concentrate on antiferromagnetic interlayer coupling $J_c>0$ as it possesses Weyl magnon nodes. The Hamiltonian is diagonalized through generalized Bogoliubov transformation. This follows by making a linear transformation $\psi_\mathbf{k}=\mathcal{P}_\mathbf{k}Q_\mathbf{k}$, where $Q_\mathbf{k}^\dagger=(b_{\mathbf{k}1}^\dagger,\, b_{\mathbf{k}2}^\dagger,\, b_{\mathbf{k}3}^\dagger, b_{-\mathbf{k}1},\, b_{-\mathbf{k}2},\, b_{-\mathbf{k}3})$ is the quasiparticle operators, and $\mathcal{P}_\mathbf{k}$ is a $2N\times 2N$ paraunitary matrix defined as

$$\mathcal{P}_\mathbf{k}=\begin{pmatrix}u_\mathbf{k} & -v_\mathbf{k}^*\\ -v_\mathbf{k} & u_\mathbf{k}^*\end{pmatrix}. \quad \text{(B13)}$$

The functions $u_\mathbf{k}$ and $v_\mathbf{k}$ are $N\times N$ matrices and they satisfy the relation

$$|u_\mathbf{k}|^2-|v_\mathbf{k}|^2=\mathbf{I}_{N\times N}. \quad \text{(B14)}$$

Whereas the paraunitary operator $\mathcal{P}_\mathbf{k}$ satisfies the relations,

$$\mathcal{P}_\mathbf{k}^\dagger\mathcal{H}(\mathbf{k})\mathcal{P}_\mathbf{k}=\mathcal{E}_\mathbf{k}, \quad \text{(B15)}$$

$$\mathcal{P}_\mathbf{k}^\dagger\boldsymbol{\tau}_3\mathcal{P}_\mathbf{k}=\boldsymbol{\tau}_3, \quad \text{(B16)}$$

where $\mathcal{E}_\mathbf{k}=\text{diag}(E_{\mathbf{k}n},E_{-\mathbf{k}n})$, $\boldsymbol{\tau}_3=\text{diag}(\mathbf{I}_{N\times N},-\mathbf{I}_{N\times N})$, $E_{\mathbf{k},n}$ are the eigenmodes for band $n$, and "diag" denotes diagonal matrix. From Eq. B16 the relation $\mathcal{P}_\mathbf{k}^\dagger=\boldsymbol{\tau}_3\mathcal{P}_\mathbf{k}^{-1}\boldsymbol{\tau}_3$ holds. Therefore, from Eq. B15 the Hamiltonian to be diagonalized is given by $\mathcal{H}_B(\mathbf{k})=\boldsymbol{\tau}_3\mathcal{H}(\mathbf{k})$, whose eigenvalues are given by $\boldsymbol{\tau}_3\mathcal{E}_\mathbf{k}$ and the columns of $\mathcal{P}_\mathbf{k}$ are the corresponding eigenvectors. For $D_p=0$ the system has U(1) rotational invariance and degenerate energy bands form nodal-line magnons (NLMs) as we have previously discussed [48].

## Appendix C: Weyl magnon bands

For $D_p\neq 0$ rotational invariance and time-reversal symmetry are explicitly broken due to noncoplanar chiral spin textures. Therefore the possibility of Weyl magnons (WMs) becomes possible as discussed in the main text. At $(k_x,k_y)=(\pm 2\pi/3,0)$ and $(k_x,k_y)=(0,0)$ the eigenvalues of $\mathcal{H}_B(\mathbf{k})$ can be found exactly as a function of $k_z$, hence the location of the WM nodes.

At $(k_x,k_y)=(\pm 2\pi/3,0)$, the magnon bands are given by

$$\begin{aligned}[E_0(k_z)]^2=\frac{1}{2}\Big[&2\{\mathcal{G}^0(k_z)\}^2+(t^r)^2-(t_c^o)^2-2(t^o)^2\\ &+4t_c^ot^o\cos(k_z)-(t_c^o)^2\cos(2k_z) \quad \text{(C1)}\\ &-4t^r\mathcal{G}^0(k_z)\cos(\phi)+(t^r)^2\cos(2\phi)\Big].\end{aligned}$$

$$\begin{aligned}[E_\pm(k_z)]^2=\frac{1}{2}\Big[&\{2\mathcal{G}^0(k_z)\}^2+2(t^r)^2-2(t_c^o)^2-(t^o)^2\\ &-2t_c^o\{2t^o\cos(k_z)+4t_c^o\cos(2k_z)\} \quad \text{(C2)}\\ &+4t^r\mathcal{G}^0(k_z)\cos(\phi)-(t^r)^2\cos(2\phi)\\ &\pm 2\sqrt{3}t^r\sin(\phi)[2\mathcal{G}^0(k_z)+t^r\cos(\phi)]\Big], \quad \text{(C3)}\end{aligned}$$

where subscript 0 denotes lowest band, whereas $\mp$ denotes middle and topmost bands respectively.

At $(k_x,k_y)=(0,0)$, the magnon bands are given by

$$\begin{aligned}[E_0(k_z)]^2=\frac{1}{2}\Big[&2\{\mathcal{G}^0(k_z)\}^2+(2t^r)^2-(t_c^o)^2-2(2t^o)^2\\ &-t_c^o\{8t^o\cos(k_z)+t_c^o\cos(2k_z)\} \quad \text{(C4)}\\ &+8t^r\mathcal{G}^0(k_z)\cos(\phi)+(2t^r)^2\cos(2\phi)\Big].\end{aligned}$$

$$\begin{aligned}[E_\pm(k_z)]^2=\frac{1}{2}\Big[&2\{\mathcal{G}^0(k_z)\}^2+(2t^r)^2-(t_c^o)^2-2(t^o)^2\\ &+t_c^o\{4t^o\cos(k_z)-t_c^o\cos(2k_z)\} \quad \text{(C5)}\\ &-4t^r\mathcal{G}^0(k_z)\cos(\phi)-2(t^r)^2\cos(2\phi)\\ &\pm 4\sqrt{3}t^r\sin(\phi)[\mathcal{G}^0(k_z)-t^r\cos(\phi)]\Big]. \quad \text{(C6)}\end{aligned}$$

The lowest and middle magnon bands cross linearly (form WM nodes) at $(\pm 2\pi/3,0,k_0^1)$ and $(0,0,k_0^2)$, where

$$k_0^1=\pm\cos^{-1}(\alpha_1/\beta_1) \quad \text{(C7)}$$

$$k_0^2=\pm\cos^{-1}(\alpha_2/\beta_2), \quad \text{(C8)}$$

$$\begin{aligned}\alpha_1=3(t^o)^2+t^r\Big[&-3t^r\cos(2\phi)+6\cos(\phi)\{-1+\sqrt{3}D_z\\ &+(3+\sqrt{3}D_z+2Jc)\cos(2\eta)+2\sqrt{3}D_p\sin(2\eta)\}\\ &-2\{-\sqrt{3}+3D_z+[3D_z+\sqrt{3}(3+2J_c)]\cos(2\eta)\\ &+\sqrt{3}t^r\cos(\phi)+6D_p\sin(2\eta)\}\sin(\phi)\Big], \quad \text{(C9)}\end{aligned}$$

$$\beta_1=12t_c^ot^o-4t^rt_c^r\big[3\cos(\phi)-\sqrt{3}\sin(\phi)\big]. \quad \text{(C10)}$$

$$\begin{aligned}\alpha_2=-3(t^o)^2+t^r\Big[&3t^r\cos(2\phi)+3\cos(\phi)\{-1+\sqrt{3}D_z\\ &+(3+\sqrt{3}D_z+2J_c)\cos(2\eta)+2\sqrt{3}D_p\sin(2\eta)\}\\ &+\{6D_z\cos^2(\eta)+\sqrt{3}(3+2J_c)\cos(2\eta)\\ &-\sqrt{3}(1+2t^r\cos(\phi))+6D_p\sin(2\eta)\}\sin(\phi)\Big], \quad \text{(C11)}\end{aligned}$$

$$\beta_2=6t_c^ot^o-2t^rt_c^r[3\cos(\phi)+\sqrt{3}\sin(\phi)]. \quad \text{(C12)}$$

The topmost and lowest magnon bands cross linearly (form WM nodes) at $(\pm 2\pi/3,0,\tilde{k}_0^1)$ and $(0,0,\tilde{k}_0^2)$, where

$$\tilde{k}_0^1=\pm\cos^{-1}(\tilde{\alpha}_1/\tilde{\beta}_1), \quad \text{(C13)}$$

$$\tilde{k}_0^2=\pm\cos^{-1}(\tilde{\alpha}_2/\tilde{\beta}_2), \quad \text{(C14)}$$

$$\tilde{\alpha}_1 = -3(t^o)^2 - t^r \Big[ - 3t^r \cos(2\phi) + 6\cos(\phi)\{-1 + \sqrt{3}D_z$$
$$+ (3 + \sqrt{3}D_z + 2Jc)\cos(2\eta) + 2\sqrt{3}D_p \sin(2\eta)\}$$
$$+ 2\{-\sqrt{3} + 3D_z + [3D_z + \sqrt{3}(3 + 2J_c)]\cos(2\eta)$$
$$+ \sqrt{3}t^r \cos(\phi) + 6D_p \sin(2\eta)\}\sin(\phi)\Big], \qquad (C15)$$

$$\tilde{\beta}_1 = -12t^o_c t^o + 4t^r t^r_c \big[\cos(\phi) + \sqrt{3}\sin(\phi)\big], \qquad (C16)$$

$$\tilde{\alpha}_2 = -3(t^o)^2 + t^r \Big[3t^r \cos(2\phi) + 3\cos(\phi)\{-1 + \sqrt{3}D_z$$
$$+ (3 + \sqrt{3}D_z + 2J_c)\cos(2\eta) + 2\sqrt{3}D_p \sin(2\eta)\}$$
$$+ \{\sqrt{3} - 3D_z - [3D_z + \sqrt{3}(3 + 2J_c)]\cos(2\eta)$$
$$+ 2\sqrt{3}t^r \cos(\phi) - 6D_p \sin(2\eta)\}\sin(\phi)\Big], \qquad (C17)$$

$$\tilde{\beta}_2 = 6t^o_c t^o - 2t^r t^r_c[3\cos(\phi) - \sqrt{3}\sin(\phi)]. \qquad (C18)$$


[1] E. H. Hall, Am. J. Math. **2**, No. 3 (1879), pp. 287-292.

[2] K. v. Klitzing, G. Dorda, and M. Pepper, Phys. Rev. Lett. **45**, 494 (1980).

[3] R. B. Laughlin, Phys. Rev. B **23**, 5632(R) (1981).

[4] D. J. Thouless, M. Kohmoto, M. P. Nightingale, and M. den Nijs, Phys. Rev. Lett. **49**, 405 (1982).

[5] M. Kohmoto, Ann. Phys. **160**, 343 (1985).

[6] K. S. Novoselov, Z. Jiang, Y. Zhang, S. V. Morozov, H. L. Stormer, U. Zeitler, J. C. Maan, G. S. Boebinger, P. Kim, A. K. Geim, Science **315**, 1379 (2007).

[7] A. Tsukazaki, A. Ohtomo, T. Kita, Y. Ohno, H. Ohno, M. Kawasaki, Science **315**, 1388 (2007).

[8] N. Nagaosa, J. Sinova, S. Onoda, A. H. MacDonald, and N. P. Ong Rev. Mod. Phys. **82**, 1539 (2010).

[9] H. Chen, Q. Niu, and A. H. MacDonald, Phys. Rev. Lett. **112**, 017205 (2014).

[10] S. Nakatsuji, N. Kiyohara, and T. Higo, Nature **527**, 212 (2015).

[11] A. K. Nayak, J. E. Fischer, Y. Sun, B. Yan, J. Karel, A. C. Komarek, C. Shekhar, N. Kumar, W. Schnelle, J. Kübler, C. Felser and S. S. P. Parkin, Sci. Adv. **2**, e1501870 (2016).

[12] N. Kiyohara, T. Tomita, and S. Nakatsuji, Phys. Rev. Applied **5**, 064009 (2016).

[13] J. Kübler and C. Felser, EPL (Europhys. Lett.) **108**, 67001 (2014).

[14] N. Ito and K. Nomura, J. Phys. Soc. Jpn. **86**, 063703 (2017).

[15] Z. H. Liu, Y. J. Zhang, G. D. Liu, B. Ding, E. K. Liu Wang, X.Q.Ma, and G.H.Wu, H. M. Jafri, Z. P. Hou, W. H. Wang, X.Q.Ma, and G.H. Wu, Scientific Reports **7**, 515 (2017).

[16] T. Suzuki, R. Chisnell, A. Devarakonda, Y.-T. Liu, W. Feng, D. Xiao, J. W. Lynn and J. G. Checkelsky, Nat. Phys. **12**, 1119 (2016).

[17] K. Ohgushi, S. Murakami, and N. Nagaosa, Phys. Rev. B **62**, R6065 (2000).

[18] Y. Taguchi, Y. Oohara, H. Yoshizawa, N. Nagaosa, and Y. Tokura, Science **291**, 2573 (2001).

[19] C. Sürgers, G. Fischer, P. Winkel and H. v. Lóhneysen, Nat. Commun **5**, 3400 (2014).

[20] Y. Machida, S. Nakatsuji, Y. Maeno, T. Tayama, T. Sakakibara, and S. Onoda, Phys. Rev. Lett. **98**, 057203 (2007).

[21] Y. Machida, S. Nakatsuji, S. Onoda, Takashi Tayama, and T. Sakakibara, Nature **463**, 210 (2008).

[22] F. D. M. Haldane, Phys. Rev. Lett. **61**, 2015 (1988).

[23] C.-Z. Chang, J. Zhang, X. Feng, J. Shen, Z. Zhang, M. Guo, K. Li, Y. Ou, P. Wei, L. -L. Wang, Z. -Q. Ji, Y. Feng, S. Ji, X. Chen, J. Jia, X. Dai, Z. Fang, S. -C. Zhang, K. He, Y. Wang, L. Lu, X. -C. Ma, Q. -K. Xue, Science **340**, 167 (2013).

[24] J. Zhou, Q. -F. Liang, H. Weng, Y. B. Chen, S. -H. Yao, Y. -F. Chen, J. Dong, G. -Y. Guo, Phys. Rev. Lett. **116**, 256601 (2016).

[25] I. Dzyaloshinsky, J. Phys. Chem. Solids **4**, 241 (1958).

[26] T. Moriya, Phys. Rev. **120**, 91 (1960).

[27] H. Katsura, N. Nagaosa, and P.A. Lee, Phys. Rev. Lett. **104**, 066403 (2010).

[28] R. Matsumoto, and S. Murakami, Phys. Rev. Lett. **106**, 197202 (2011).

[29] R. Matsumoto, and S. Murakami, Phys. Rev. B **84**, 184406 (2011).

[30] R. Matsumoto, R. Shindou, and S. Murakami, Phys. Rev. B **89**, 054420 (2014).

[31] A. Mook, J. Henk, and I. Mertig, Phys. Rev. B **89**, 134409 (2014).

[32] H. Lee, J. H. Han, and P. A. Lee, Phys. Rev. B. **91**, 125413 (2015).

[33] J. Romhányi, K. Penc, and R. Ganesh, Nat. Commun. **6**, 6805 (2015).

[34] P. A. McClarty et al., Nat. Phys., **13**, 736 (2017).

[35] Y. Onose, T. Ideue, H. Katsura, Y. Shiomi, N. Nagaosa, and Y. Tokura, Science **329**, 297 (2010).

[36] T. Ideue, Y. Onose, H. Katsura, Y. Shiomi, S. Ishiwata, N. Nagaosa, and Y. Tokura, Phys. Rev. B. **85**, 134411 (2012).

[37] M. Hirschberger, R. Chisnell, Y. S. Lee, and N. P. Ong, Phys. Rev. Lett. **115**, 106603 (2015).

[38] M. Hirschberger, J. W. Krizan, R. J. Cava, and N. P. Ong, Science **348**, 106 (2015).

[39] D. Watanabe, K. Sugii, M. Shimozawa, Y. Suzuki, T.

Yajima, H. Ishikawa, Z. Hiroi, T. Shibauchi, Y. Matsuda, M. Yamashita, Proc. Natl. Acad. Sci. USA **113**, 8653 (2016).
[40] T. Ideue, T. Kurumaji, S. Ishiwata, and Y. Tokura, Nat. Mater. **16**, 797 (2017).
[41] M. Elhajal, B. Canals, and C. Lacroix, Phys. Rev. B **66**, 014422 (2002).
[42] D. Grohol, K. Matan, J. -H. Cho, S. -H. Lee, J. W. Lynn, D. G. Nocera, and Y. S. Lee, Nat. Mater. **4**, 323 (2005).
[43] X. G. Zheng, T. Mori, K. Nishiyama, W. Higemoto, H. Yamada, K. Nishikubo, and C. N. Xu, Phys. Rev. B **71**, 174404 (2005).
[44] X. G. Zheng, H. Kubozono, K. Nishiyama, W. Higemoto, T. Kawae, A. Koda, and C. N. Xu, Phys. Rev. Lett. **95**, 057201 (2005).
[45] T. -H. Han, J. Singleton, and J. A. Schlueter, Phys. Rev. Lett. **113**, 227203 (2014).
[46] T. -H. Han, E. D. Isaacs, J. A. Schlueter, and J. Singleton, Phys. Rev. B **93**, 214416 (2016).
[47] A. Scheie, M. Sanders, J. Krizan, Y. Qiu, R. J. Cava, and C. Broholm, Phys. Rev. B **93**, 180407(R) (2016).
[48] S. A. Owerre, See Main Text.
[49] F. -Y. Li, Y. -D. Li, Y. B. Kim, L. Balents, Y. Yu, and G. Chen, Nat. Commun.**7**, 12691 (2016).
[50] S. -K. Jian, and W. Nie, arXiv:1708.02948 (2017).
[51] P. Laurell, and G. A. Fiete, Phys. Rev. Lett. **118**, 177201 (2017).
[52] A. Mook, J. Henk, and I. Mertig, Phys. Rev. Lett. **117**, 157204 (2016).
[53] S. Ying, X. S. Wang, and X. R. Wang, Phys. Rev. B **95**, 224403 (2017).
[54] Similarly, electronic Weyl nodes close to the Fermi energy are the most important ones that make significant contributions to the low-temperature transport properties.
[55] K. -Y. Yang, Y. -M. Lu, and Y. Ran, Phys. Rev. B **84**, 075129 (2011).
[56] A. A. Burkov, Phys. Rev. Lett. **113**, 187202 (2014).
[57] S. A. Owerre, Phys. Rev. B **95**, 014422 (2017).
[58] L. Zhang, J. Ren, J. -S. Wang, and B. Li, Phys. Rev. B **87**, 144101 (2013).
[59] A. Mook, J. Henk, and I. Mertig, Phys. Rev. B **90**, 024412 (2014).
[60] R. Chisnell, J. S. Helton, D. E. Freedman,D. K. Singh, R. I. Bewley, D. G. Nocera, and Y. S. Lee, Phys. Rev. Lett. **115**, 147201 (2015).
[61] T. Yildirim and A. B. Harris, Phys. Rev. B **73**, 214446 (2006).
[62] T. Ono, K. Matan, Y. Nambu, T. J. Sato, K. Katayama, S. Hirata, and H. Tanaka, J. Phys. Soc. Jpn. **83**, 043701 (2014).
